# Supplementary material for: Dynamical resonance quench and Fano interference in spontaneous Raman scattering from quasiparticle and collective excitations
Source: arXiv:1806.05986 ancillary file (2019-02-07)
Supplement: Supplementary file 1 [file SupplementaryMaterialDynamic.pdf]

*Supplemental Material for*

# Dynamical resonance quench and Fano interference in spontaneous Raman scattering from quasiparticle and collective excitations

J. Zhu[1], R. B. Versteeg[1], P. Padmanabhan[1], and P. H. M. van Loosdrecht[1]*

[1] II. Physikalisches Institut, Universität zu Köln, Zülpicher Straße 77, D-50937 Köln, Germany

*Email: pvl@ph2.uni-koeln.de

## I. Carrier density calibration by laser parameters and Fano interference

The carrier density ($\Delta c$) created by the laser excitation can be estimated by

$$\Delta c = \frac{(1-R)E}{\pi w^2 L h\nu} \quad (1),$$

where R is the reflectivity of silicon (R ~ 0.35 at 740 nm), $E$ is the pulse energy, $L$ is the optical penetration depth ($L$~ 1/1500 cm at 740 nm), and $\boldsymbol{w}$ is the laser beam radius size at the focus position on the sample surface, which is measured to be ~ 20 μm. $h$ is the Planck constant, and $\nu$ is the laser frequency. With these parameters the excited carrier density is estimated to be $1.2\times 10^{19}$ cm $^{-3}$ for an excitation pulse energy of 40 nJ at 740 nm. We use this value to linearly calibrate carrier densities generated at different excitation laser energies.

Fano interference on absorption line shapes was discussed in Fano's earlier publications.[1,2] Similar discrete and continuum states interference was also observed in steady-state Raman scattering of heavily doped silicon, [3-6] and was interpreted as interference between electronic and phonon transitions. The observed Fano interference in the phonon scattering is strongly influenced by the Raman probe wavelength and chemically doped carrier densities. Here we observe an optical excitation induced Fano effect. We plot the fitted Fano

parameters $q$ after excitation (10 ps) versus the calculated carrier density estimated by using formula (1), and compare it with the case of chemically doped silicon measurements.[4,6] As shown in Fig. S1 (a), the $q$ parameters fall within the same carrier density region as those observed from steady-state Raman measurements on chemically doped silicon. This indicates that the carrier density injected by optical excitation in pure silicon has the similar effect as that in the chemically doped case. The optically induced Fano interface thus could also be used as a calibration of carrier density generated by laser pulses. In addition, as indicated in Fig. S1 (b), the value of $1/q$ is linearly proportional to the laser doped hole density.

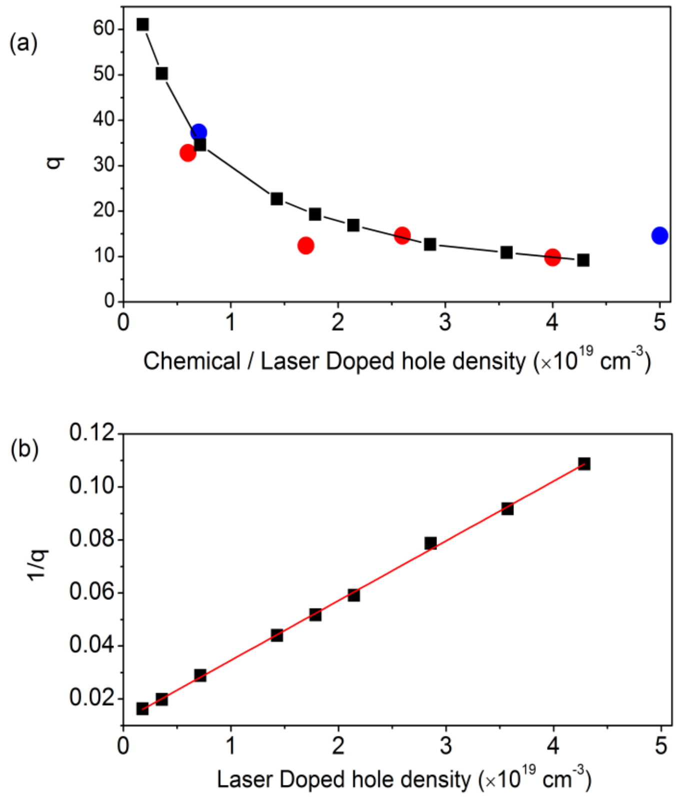


**FIG. S1. (a) Carrier density dependence of Fano parameter q in chemically p-doped silicon and in laser excited pure silicon. Red circle dots are from ref 4, in which Raman pulses have a wavelength of 488 nm, and blue circle dots are from ref 6, using 532 nm as a Raman pulse. Black square dots are from our experimental fit results with probe wavelength at 512 nm. (b) $q^{-1}$ versus carrier density generated with pulsed laser excitation.**

## II. Reflectivity changes of silicon upon optical excitation

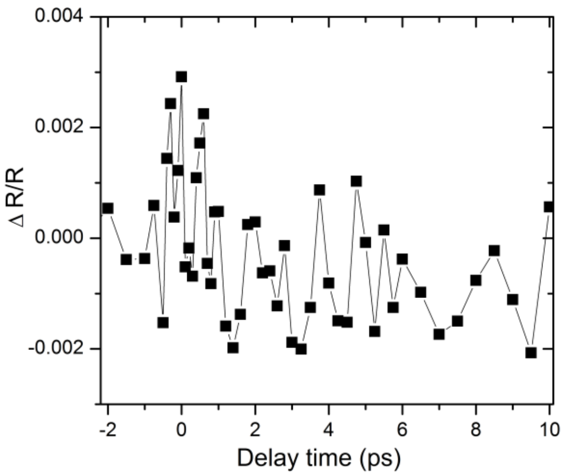


**FIG. S2 Time-resolved reflectivity changes of silicon upon excitation with 740 nm and probe at 512 nm. The excited carrier density is around $2 \times 10^{19}$ cm $^{-3}$. The change is less than 0.2% at long delay times.**

## III. Phonon Dynamics of silicon observed with 2.7 eV (450 nm) Raman probe pulse

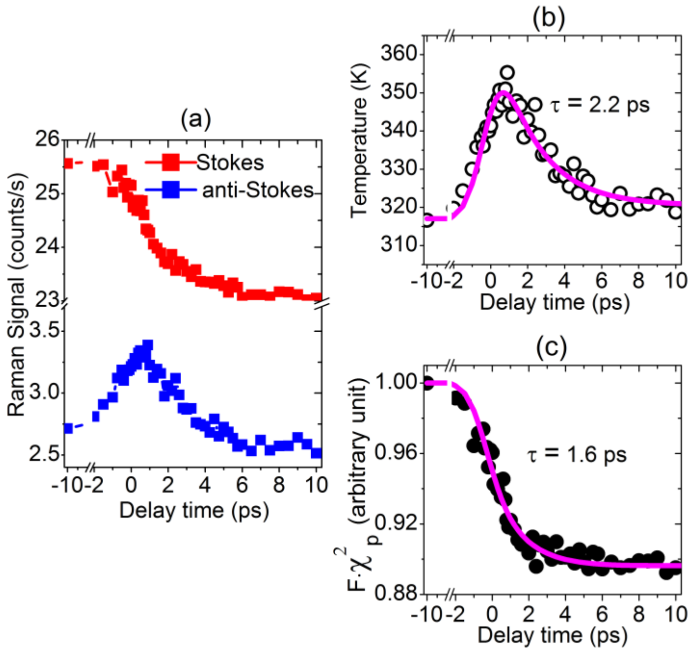


**FIG. S3 Relaxation dynamics using Raman probe pulse energy at 2.7 eV (450 nm), at the excited carrier density ~2 × 10$^{19}$ cm $^{-3}$. (a) Decay of the optical phonon intensity for Stokes scattering (red dots) and anti-Stokes scattering (blue dots). (b) Extracted phonon temperature evolution. (c) Extracted Raman scattering strength behavior with time.**

## IV. Raman tensor changes due to electronic population.

Without loss of generality, we write down the electronic susceptibility tensor $\chi_{ij}$ [7] of a two-energy level system as:

$$\chi_{ij} \propto N(\rho_{00} - \rho_{11}) \left( \frac{\langle \psi_0 | r_i | \psi_1 \rangle \langle \psi_1 | r_j | \psi_0 \rangle}{\omega_{01} - \omega - i\Gamma} + \frac{\langle \psi_0 | r_j | \psi_1 \rangle \langle \psi_1 | r_i | \psi_0 \rangle}{\omega_{01} + \omega + i\Gamma} \right) \ldots\ldots\ldots\ldots\ldots\ldots\ldots\ldots \text{(2)},$$

where N represents the atom density of the system, and $\rho_{00}$ and $\rho_{11}$ are the diagonal density matrix elements referring to the ground state $\psi_0$ and excited state $\psi_1$, $\omega$ is the laser excitation

frequency, and $\Gamma$ is the damping constant. The Raman susceptibility tensor associated with a general vibration model Q can be written as:

$$\frac{\partial \chi_{ij}}{\partial Q}|_{Q_0} \propto N(\rho_{00}-\rho_{11})\frac{\partial}{\partial Q}\left(\frac{\langle\psi_0|r_i|\psi_1\rangle\langle\psi_1|r_j|\psi_0\rangle}{\omega_{01}-\omega-i\Gamma}+\frac{\langle\psi_0|r_j|\psi_1\rangle\langle\psi_1|r_i|\psi_0\rangle}{\omega_{01}+\omega+i\Gamma}\right)|_{Q_0} \ldots\ldots\ldots\ldots (3).$$

Thus, the Raman tensor is proportional to the population difference $N(\rho_{00}-\rho_{11})$, as is the electronic susceptibility tensor, *i.e.*,

$$\frac{\partial \chi_{ij}}{\partial Q}|_{Q_0} \propto N(\rho_{00}-\rho_{11}) \ldots\ldots\ldots\ldots (4).$$

With

$$\rho_{00}+\rho_{11}=1 \ldots\ldots\ldots\ldots (5),$$

(4) becomes:

$$|\frac{\partial \chi_{ij}}{\partial Q}|_{Q_0}{}^2 \propto N(1-4\rho_{11}+4{\rho_{11}}^2) \ldots\ldots\ldots\ldots (6).$$

Since $\rho_{11} \ll 1$, the term ${\rho_{11}}^2$, can be dropped such that,

$$|\frac{\partial \chi_{ij}}{\partial Q}|_{Q_0}{}^2 \propto N(1-4\rho_{11}) \ldots\ldots\ldots\ldots (7).$$

Finally,

$$\Delta|\frac{\partial \chi_{ij}}{\partial Q}|_{Q_0}{}^2 \propto -4\mathrm{N}\rho_{11} \ldots\ldots\ldots\ldots (8).$$

*I.e.*, the reduction of the squared Raman susceptibility tensor $|\frac{\partial \chi_{ij}}{\partial Q}|_{Q_0}{}^2$ is linearly proportional to 4 times the population $\mathrm{N}\rho_{11}$.

## V. References

[1] U. Fano, G. Pupillo, A. Zannoni, and C. W. Clark, J. Res. Natl. Inst. Stan. **110**, 583 (2005).

[2] U. Fano, Phys. Rev. **124**, 1866 (1961).

[3] F. Cerdeira, T. A. Fjeldly, and M. Cardona, Solid State Commun. **13**, 325 (1973).

[4] F. Cerdeira, T. A. Fjeldly, and M. Cardona, Phys. Rev. B **8**, 4734 (1973).

[5] M. Chandrasekhar, J. B. Renucci, and M. Cardona, Phys. Rev. B **17**, 1623 (1978).

[6] B. G. Burke, J. Chan, K. A. Williams, Z. L. Wu, A. A. Puretzky, and D. B. Geohegan, J. Raman Spectrosc. **41**, 1759 (2010).

[7] R. W. Boyd, in *page 163, chapter 3, Quantum-Mechanical Theory of the Nonlinear Optical Susceptibility* in *Nonlinear optics,* 3rd ed. (Elsevier, Amsterdam , 2008).
